# Supplementary material for: GRAFT: Graph-Regularized Prototype Fields for Realistic Test-Time Adaptation of VLMs
Source: arXiv:2611.23591 source file (2026-11-17)
Supplement: Supplementary file 1 [file X_suppl.tex]

\section{Proofs}
\label{sec:proofs}
Throughout, $Q_\lambda = \alpha I + \lambda L_T$, $N_z = \diag(n)$, and for a fixed feature dimension $j$ we write $d = d_{:j}$, $e = e_{:j}$ and $s = s_j$.

\paragraph{Derivation of \cref{eq:dsolve}.}
Given $z$, the terms of \cref{eq:objective} that depend on $D$ are $\sum_{i,k} z_{ik}\frac{(x_{ij} - t_{kj} - d_{kj})^2}{2\kappa\sigma_j^2}$ summed over $j$, plus $\frac{1}{2\kappa\bar\sigma^2}\sum_j d_{:j}^{\top}Q_\lambda d_{:j}$. Expanding the square around $\bar{x}_{kj}$ and dropping terms that do not depend on $d$ gives, per dimension, $\frac{1}{2\kappa\sigma_j^2}\sum_k n_k (d_k - e_k)^2 + \frac{1}{2\kappa\bar\sigma^2} d^{\top}Q_\lambda d$. Multiplying by $\kappa\sigma_j^2$ and setting the gradient to zero yields $(N_z + s_j Q_\lambda)d = N_z e$, which is \cref{eq:dsolve}. The matrix is positive definite whenever $\alpha>0$ or $n_k>0$ for some $k$ in every connected component, so the solution is unique.

\paragraph{Proof of the special cases (\cref{sec:field}).}
With $\lambda=0$ the system is diagonal: $(n_k + s\alpha)d_k = n_k e_k$. With $\alpha = 0$ and $L_T$ the normalised Laplacian of the complete graph, $L_T = \frac{K}{K-1}(I - \frac{1}{K}\mathbf{1}\mathbf{1}^{\top})$, whose null space is spanned by $\mathbf{1}$. As $\lambda\to\infty$ the minimiser of $\frac12\sum_k n_k(d_k-e_k)^2 + \frac{\lambda s}{2}d^{\top}L_Td$ is forced into the null space, $d = \delta\mathbf{1}$, and minimising over $\delta$ gives $\delta = \sum_k n_k e_k/\sum_k n_k$. \qed

\paragraph{Proof of the harmonic-extension property (\cref{sec:field}).}
Partition the system by $A$ and $P$. Rows in $A$ have $n_k = 0$ and $e_k = 0$, so they read $s\,(Q_{\lambda,AA}d_A + Q_{\lambda,AP}d_P) = 0$, which gives the harmonic extension $d_A = -Q_{\lambda,AA}^{-1}Q_{\lambda,AP}d_P$ ($Q_{\lambda,AA}$ is positive definite when $\alpha>0$, or when every component of $A$ touches $P$). Substituting into the $P$ rows gives $(N_{z,P} + s(Q_{\lambda,PP} - Q_{\lambda,PA}Q_{\lambda,AA}^{-1}Q_{\lambda,AP}))d_P = N_{z,P}e_P$, which is \cref{eq:dsolve} on $P$ with the Schur complement $Q_\lambda/Q_{\lambda,AA}$, the Kron reduction of the graph onto $P$~\cite{dorfler2013kron}. \qed

\paragraph{Proof of the posterior-variance bound (\cref{sec:field}).}
Given $z$, the per-dimension posterior of $d$ is Gaussian with precision $(N_z + sQ_\lambda)/(\kappa\sigma_j^2)$, so its covariance is $\kappa\sigma_j^2(N_z + sQ_\lambda)^{-1}$. For symmetric positive definite $A$ and positive semi-definite $B$, $(A+B)^{-1}\preceq A^{-1}$, hence the diagonal entries satisfy $[(N_z + s\alpha I + s\lambda L_T)^{-1}]_{kk}\le [(N_z + s\alpha I)^{-1}]_{kk} = 1/(n_k + s\alpha)$. Strictness: $[(A+B)^{-1}]_{kk} = [A^{-1}]_{kk}$ for all $k$ in a set $C$ would require $B$ to vanish on the corresponding block of the Woodbury expansion, which fails for any class $k$ with $(L_T)_{kk}>0$, that is, any class with at least one neighbour. \qed

\paragraph{Proof of monotone block updates (\cref{sec:inference}).}
With $\lambda_L = 0$ the objective is, in $z$, a sum of $N$ strictly convex functions on the simplex whose minimisers are the softmax in \cref{eq:estep} (standard mean-field argument), in $\pi$ a Dirichlet-regularised multinomial likelihood whose minimiser is \cref{eq:pi}, in $D$ a strictly convex quadratic (above) and in $\sigma^2$ a separable problem whose stationary point is the stated variance. Each block update therefore does not increase $J$, which is bounded below, so $J$ converges. With $\lambda_L>0$ the term $-\frac{\lambda_L}{2m_s}z^{\top}W_s z$ is handled by the linear bound $-z^{\top}W_s z\le -2 z^{\top}W_s z^{(t)} + z^{(t)\top}W_s z^{(t)}$, valid when $W_s$ is positive semi-definite and used as a majoriser otherwise, as in~\cite{ziko2020laplacianshot,zanella2024transclip}. \qed

\section{Batch and online algorithms}
\begin{algorithm}[h]
\caption{\method, batch (transductive) inference}
\label{alg:batch}
\begin{algorithmic}[1]
\Require features $X\in\R^{N\times d}$, anchors $T\in\R^{K\times d}$, graph $L_T$, $(\alpha,\lambda)$ or empirical Bayes, $c$, $\kappa$, $\lambda_y$, $\lambda_L$
\State $\hat{y}\gets\mathrm{softmax}(\tau XT^{\top})$; $z\gets\hat{y}$; $D\gets 0$; $\pi\gets\mathbf{1}/K$; $\sigma^2\gets$ variance of $X$ about $T$ under $\hat{y}$
\State $W_s\gets$ $m_s$-NN cosine graph of $X$
\For{$t=1,\dots,T_{\max}$}
  \State E-step: update $z$ by \cref{eq:estep} ($n_{\mathrm{inner}}$ sweeps)
  \State $n\gets z^{\top}\mathbf{1}$;\; $\bar{X}\gets N_z^{-1}z^{\top}X$;\; $E\gets\bar{X}-T$ (rows with $n_k=0$ set to $0$)
  \State $\pi\gets(n+c)/(N+Kc)$ \Comment{presence}
  \State optionally $(\alpha,\lambda)\gets\argmax$ marginal likelihood of $E$ (\cref{sec:eb})
  \State $D\gets$ solution of \cref{eq:dsolve} \Comment{graph-pooled field}
  \State $\sigma_j^2\gets\tfrac{1}{N}\big[q_j - 2\sum_k\mu_{kj}S_{kj} + \sum_k n_k\mu_{kj}^2\big]$ with $\mu=T+D$
\EndFor
\State \Return $z$ (posterior), $(D,\pi,\sigma^2)$
\end{algorithmic}
\end{algorithm}

\begin{algorithm}[h]
\caption{\method, online inference on a stream}
\label{alg:online}
\begin{algorithmic}[1]
\Require anchors $T$, graph $L_T$, forgetting $\varrho\in(0,1]$; state $(n,S,q,N)\gets 0$, $D\gets 0$, $\pi\gets\mathbf{1}/K$
\For{each batch $X^{(b)}$}
  \State $\hat{y}\gets\mathrm{softmax}(\tau X^{(b)}T^{\top})$; E-step with current $(D,\pi,\sigma^2)$ \Cref{eq:estep}
  \State $(n,S,q,N)\gets\varrho\,(n,S,q,N) + \big(z^{\top}\mathbf{1},\, z^{\top}X^{(b)},\, \textstyle\sum_i x_i^{\odot2},\, |X^{(b)}|\big)$
  \State M-steps of \cref{alg:batch} from $(n,S,q,N)$; re-run the E-step on $X^{(b)}$ (two rounds)
  \State \Return posterior $z$ of $X^{(b)}$
\EndFor
\end{algorithmic}
\end{algorithm}

\section{Empirical Bayes details}
Given the responsibilities, the empirical displacements of the present classes $P=\{k: n_k\ge 1\}$ are, under the model, $e_P = d_P + \epsilon$ with $\epsilon_k\sim\mathcal{N}(0,\kappa\sigma^2/n_k)$ and $d_P\sim\mathcal{N}(0,\tilde{Q}_P^{-1})$, where $\tilde{Q}_P$ is the Schur complement of $Q$ onto $P$. With the isotropic approximation $\sigma_j^2\approx\bar\sigma^2$, the marginal likelihood of $E_P$ is a Gaussian with covariance $C=\kappa\bar\sigma^2(\tilde{Q}_P^{-1}+N_{z,P}^{-1})$ per dimension,
\begin{equation}
  \log p(E_P\,|\,\alpha,\lambda) = -\tfrac{1}{2}\tr\big(E_P^{\top}C^{-1}E_P\big) - \tfrac{d}{2}\log\det C + \mathrm{const},
  \label{eq:evidence}
\end{equation}
which is maximised over the grid $\alpha\in\{0.25,\dots,8\}$, $\lambda\in\{0,1,\dots,32\}$.
With $P$ the present classes, the marginal covariance of $e_{:j,P}$ in pseudo-count units is $\tilde{Q}_P^{-1} + N_{z,P}^{-1}$ where $\tilde{Q}_P$ is the Schur complement of $Q_\lambda$ onto $P$, because marginalising a GMRF onto a subset of nodes replaces the precision by its Schur complement~\cite{rue2005gmrf}. The evidence of \cref{eq:evidence} sums the $d$ independent dimensions after whitening $E$ by $\sqrt{\kappa\bar\sigma^2}$. One Cholesky factorisation of a $|P|\times|P|$ matrix per grid point suffices; the Schur complement requires one solve with $Q_{\lambda,AA}$, which is sparse and well conditioned when $\alpha>0$. The rule is disabled when $|P|<3$, since the evidence is then nearly flat in $\lambda$.

\section{Datasets and protocol details}

\begin{table}[h]
  \centering\footnotesize
  \caption{Benchmarks (CoOp test splits). $K$: vocabulary size; $N_{\mathrm{test}}$: number of test images.}
  \label{tab:datasets}
  \setlength{\tabcolsep}{3pt}
  \begin{tabular}{lrr@{\hskip 8pt}lrr}
    \toprule
    Dataset & $K$ & $N_{\mathrm{test}}$ & Dataset & $K$ & $N_{\mathrm{test}}$\\
    \midrule
    ImageNet & 1000 & 50,000 & Oxford Pets & 37 & 3,669\\
    SUN397 & 397 & 19,850 & Flowers102 & 102 & 2,463\\
    FGVC-Aircraft & 100 & 3,333 & Caltech101 & 100 & 2,465\\
    EuroSAT & 10 & 8,100 & DTD & 47 & 1,692\\
    Stanford Cars & 196 & 8,041 & UCF101 & 101 & 3,783\\
    Food101 & 101 & 30,300 & ImageNet-V2 / S & 1000 & 10,000 / 50,889\\
     & & & ImageNet-A / R & 200 & 7,500 / 30,000\\
    \bottomrule
  \end{tabular}
\end{table}

The batch sampler draws $K_{\mathrm{eff}}$ uniformly in $[k_{\min},k_{\max}]$, selects $K_{\mathrm{eff}}$ classes without replacement, pools their test images and draws $B$ of them without replacement (all of them if fewer than $B$ are available). The online sampler draws, for each class, Dirichlet($\gamma$) proportions over $K$ slots, assigns the class's shuffled images to slots accordingly, shuffles within slots and concatenates the slots; $\gamma=-1$ denotes the separate stream. These re-implementations follow the description of~\cite{zanella2025stata}; the released adapter also runs \method inside the official harness so that the exact official samplers can be used.

\section{Hyper-parameters}
\begin{table}[h]
  \centering\small
  \begin{tabular}{llc}
    \toprule
    Symbol & Meaning & Value\\
    \midrule
    $\tau$ & logit scale of the VLM & 100\\
    $\kappa$ & likelihood temperature (inherited) & 50\\
    $\lambda_y$ & exponent of the zero-shot prior (inherited) & 1\\
    $\lambda_L$, $m_s$ & sample-graph weight and neighbours (inherited) & 1, 3\\
    $\alpha$ & anchor strength (pseudo-counts) & 1\\
    $\lambda$ & graph coupling (pseudo-counts) & 4\\
    $m$, $\rho$ & class-graph neighbours and bandwidth & 5, 0.05\\
    $c$ & Dirichlet pseudo-count of $\pi$ & 0.5\\
    $T_{\max}$, $n_{\mathrm{inner}}$ & outer and inner iterations & 10, 3\\
    $n_{\mathrm{cg}}$ & conjugate-gradient iterations & 30\\
    $\varrho$ & online forgetting factor & 1 (none)\\
    \bottomrule
  \end{tabular}
\end{table}


\section{Mechanism on synthetic data}
\begin{figure}[h]
  \centering
  \includegraphics[width=\linewidth]{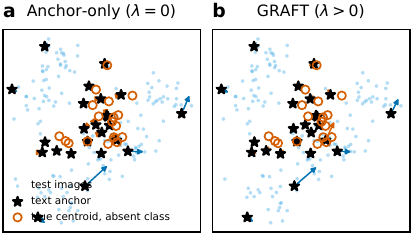}
  \caption{Adapted prototypes on synthetic data (6 of 24 classes present, PCA to two dimensions). Arrows go from text anchors to adapted prototypes; orange marks absent classes and circles their true centroids.}
  \label{fig:embed}
\end{figure}
\noindent With $\lambda=0$ absent classes stay at their anchors, whereas the pooled field moves them towards the centroids their images would occupy.

\section{Prior and graph ablation}
\begin{table}[h]
  \centering
  \caption{Prior and graph ablation in the low setting (default: $\alpha{=}1$, $\lambda{=}4$, $m{=}5$, $\rho{=}0.05$). Standard deviations over tasks are 0.3 for every entry.}
  \label{tab:prior}
  \footnotesize\setlength{\tabcolsep}{2.5pt}
  \begin{tabular}{@{}lcccccc@{}}
    \toprule
    $\alpha$ & 0 & 0.25 & 1 & 4 & 16 & \\
    acc. & \ph{69.0} & \ph{70.2} & \ph{\textbf{70.7}} & \ph{70.4} & \ph{69.6} & \\
    \midrule
    $\lambda$ & 0 & 1 & 4 & 16 & 64 & $\infty$\\
    acc. & \ph{69.1} & \ph{70.1} & \ph{\textbf{70.7}} & \ph{70.5} & \ph{69.9} & \ph{68.8}\\
    \midrule
    graph & $m{=}3$ & $m{=}5$ & $m{=}10$ & compl. & rand. & \\
    acc. & \ph{70.4} & \ph{\textbf{70.7}} & \ph{70.5} & \ph{68.8} & \ph{69.2} & \\
    \bottomrule
  \end{tabular}
\end{table}

\section{Smoothness and sensitivity plots}
\begin{figure}[h]
  \centering
  \includegraphics[width=\linewidth]{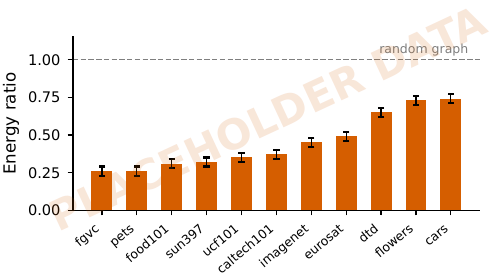}
  \caption{Class-level smoothness: Dirichlet energy of the oracle displacement field on the text graph relative to degree-matched random graphs (lower is smoother; error bars: standard deviation over 20 random graphs).}
  \label{fig:smooth}
\end{figure}

\begin{figure}[h]
  \centering
  \includegraphics[width=\linewidth]{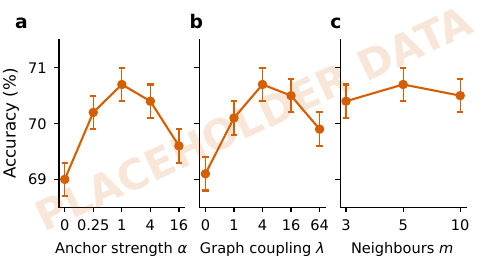}
  \caption{Sensitivity to the prior strengths and the graph size in the low setting (mean and standard deviation over tasks).}
  \label{fig:sens}
\end{figure}

\section{Additional result tables}
\begin{table}[h]
  \centering\footnotesize
  \caption{Backbones and distribution shifts, low setting ($B{=}64$, $K_{\mathrm{eff}}\in[2,10]$), top-1 accuracy (\%). IN: ImageNet; V2/S/A/R: its shifted variants.}
  \label{tab:backbones}
  \begin{tabular}{llccccc}
    \toprule
    Backbone & Method & IN & V2 & S & A & R\\
    \midrule
    \multirow{3}{*}{CLIP ViT-B/16} & zero-shot & \TBD & \TBD & \TBD & \TBD & \TBD\\
     & StatA & \TBD & \TBD & \TBD & \TBD & \TBD\\
     & \method & \TBD & \TBD & \TBD & \TBD & \TBD\\
    \multirow{3}{*}{CLIP ViT-L/14} & zero-shot & \TBD & \TBD & \TBD & \TBD & \TBD\\
     & StatA & \TBD & \TBD & \TBD & \TBD & \TBD\\
     & \method & \TBD & \TBD & \TBD & \TBD & \TBD\\
    \multirow{3}{*}{OpenCLIP B/16} & zero-shot & \TBD & \TBD & \TBD & \TBD & \TBD\\
     & StatA & \TBD & \TBD & \TBD & \TBD & \TBD\\
     & \method & \TBD & \TBD & \TBD & \TBD & \TBD\\
    \multirow{3}{*}{SigLIP B/16} & zero-shot & \TBD & \TBD & \TBD & \TBD & \TBD\\
     & StatA & \TBD & \TBD & \TBD & \TBD & \TBD\\
     & \method & \TBD & \TBD & \TBD & \TBD & \TBD\\
    \bottomrule
  \end{tabular}
\end{table}

\begin{table}[h]
  \centering\footnotesize
  \caption{Trustworthiness in the low setting ($B{=}64$), averaged over eleven datasets, CLIP ViT-B/16. ECE and NLL: lower is better; worst-decile accuracy: higher is better.}
  \label{tab:calib}
  \begin{tabular}{lccc}
    \toprule
    Method & ECE (\%) $\downarrow$ & NLL $\downarrow$ & Worst-decile acc. (\%) $\uparrow$\\
    \midrule
    CLIP zero-shot & \TBD & \TBD & \TBD\\
    TransCLIP & \TBD & \TBD & \TBD\\
    StatA & \TBD & \TBD & \TBD\\
    MOON & \TBD & \TBD & \TBD\\
    Anchor-only control & \TBD & \TBD & \TBD\\
    \method & \TBD & \TBD & \TBD\\
    \bottomrule
  \end{tabular}
\end{table}

\begin{table}[h]
  \centering\footnotesize
  \caption{Likelihood, optimisation and cost, low setting. Time is the wall-clock per task of 64 images on one GPU with cached features (ImageNet, $K{=}1000$).}
  \label{tab:opt}
  \begin{tabular}{lcc}
    \toprule
    Variant & acc. (\%) & time (ms)\\
    \midrule
    default (shared diagonal $\Sigma$, no re-projection, $c{=}0.5$, $\kappa{=}50$, $T_{\max}{=}10$) & \TBD & \TBD\\
    isotropic $\Sigma$ & \TBD & \TBD\\
    per-class diagonal $\Sigma_k$ (as StatA) & \TBD & \TBD\\
    re-project $\mu_k$ onto the sphere & \TBD & \TBD\\
    $c\in\{0.1, 2\}$ & \TBD / \TBD & \\
    $\kappa\in\{25, 100\}$ & \TBD / \TBD & \\
    $T_{\max}\in\{3, 20\}$ & \TBD / \TBD & \TBD / \TBD\\
    exact solver instead of conjugate gradients & \TBD & \TBD\\
    \bottomrule
  \end{tabular}
\end{table}

\begin{table}[h]
  \centering\footnotesize
  \caption{Computational cost: asymptotic cost per outer iteration and measured time per task ($B{=}64$, ImageNet, one GPU).}
  \label{tab:cost}
  \begin{tabular}{lll}
    \toprule
    Method & dominant cost & ms / task\\
    \midrule
    zero-shot & $O(NKd)$ & \TBD\\
    TransCLIP & $O(NKd + Nm_sK)$ & \TBD\\
    StatA & $O(NKd + Nm_sK)$ & \TBD\\
    MOON & $O(NKd + Nm_sK)$ & \TBD\\
    \method (CG) & $O(NKd + Nm_sK + n_{\mathrm{cg}}Kd(1+m))$ & \TBD\\
    \method + EB & above $+\,O(|G|K^3)$ & \TBD\\
    \bottomrule
  \end{tabular}
\end{table}

\section{Per-dataset results}
Per-dataset versions of the main tables are generated by the released scripts (\texttt{visualization/generate\_tables.py}) and will be included here once the runs complete.
